# Supplementary material for: Agents meet OKR: An Object and Key Results Driven Agent System with Hierarchical Self-Collaboration and Self-Evaluation
Source: arXiv:2311.16542 source file (2023-11-28)
Supplement: Supplementary file 1 [file appendix.tex]

\section{Appendix}

\subsection{Short Video StoryBoard Writing}

\begin{table}[h]
  \centering
  \includegraphics[width=1.0\textwidth]{figures/调研表格A.png}
  \tiny
  \caption{Subjective Evaluation of Comparative Experiment on Text-to-Image Generation}
  \label{fig:OKR-DramaTron2}
\end{table}

\subsection{Trivia Creative Writing task example}

\paragraph{Story}
In this scene, the camera looks down from a distant height, revealing the vast continent of Hyrule. Distant mountains stand tall, lush trees dot the land, and a clear stream winds its way through. It is now the evening, with the gentle glow of the setting sun casting a serene and mysterious atmosphere over the continent.
The protagonist, Ed Stark, exudes an air of mystery and confidence as he strides into Hyrule from the edge of the grassy area. His gaze is resolute and sharp, conveying excitement and curiosity for the unknown world. While there is no overt interaction between the characters, the audience can feel the exchange and collision between the protagonist and the environment.
At this moment, Ed Stark doesn't speak, but his eyes reveal determination and passion. The background music seamlessly blends a soft piano melody with Jay Chou's song "Silence," creating a tranquil yet mysterious ambiance. The chirping of birds and the sound of flowing water artfully merge into the music, adding vividness and a touch of nature to the scene.

The scene begins from a high vantage point, showcasing a dense forest. The camera weaves through the trees, revealing the dimly lit surroundings, with thick foliage obscuring the sky. It is now evening, and the lingering glow of the setting sun filters through the leaves, creating dappled patterns of light and shadow on the ground.
Ed swiftly wields his wand, moving nimbly between the trees. Each of his actions demonstrates exquisite combat skills and unwavering determination. His face carries a resolute expression, with furrowed brows and sharp eyes revealing his determination and intense focus.
The protagonist follows closely, attempting to keep pace with Ed's strides, but appears somewhat awkward in the dense forest.
Ed softly chants the incantation "Expecto Patronum," his voice gentle yet firm. A mysterious and exhilarating music gradually begins, emphasizing the tense yet hopeful atmosphere.
The rustling of leaves and distant insect chirping intertwine, creating an air of mystery in the forest.

The camera transitions from a long shot to a close-up, highlighting the twisted energy of the Dark Zone. This area is shrouded in heavy shadows, resembling a suspended dark cloud, pitch black and filled with an aura of terror and mystery. It is nighttime, and the bright moon hangs high above the Dark Zone, adding a touch of chilling elegance and mystique.
The protagonist and Ed grip their weapons tightly, maintaining a vigilant stance, preparing for an intense battle against the forces of darkness. The protagonist wields a radiant magical sword, with each strike releasing dazzling light. Ed's magic wand emits sparks of electricity, shattering the encroaching shadows. Their gaze is resolute, revealing a determination to combat evil. They remain focused and alert, driven by a pursuit of justice.
Amidst the fierce battle, they exchange dialogue:
Protagonist: "Ed, together we will conquer the darkness!"
Ed responds: "No problem! Our power will annihilate the malevolence!"
The music swells with passionate melodies, reaching crescendos alongside the protagonist and Ed's confrontation, adding depth to the battle.

The camera overlooks from a high vantage point, revealing the magnificent spectacle of the entire Hyrule. Beautiful and grand, Hyrule is characterized by undulating mountains, azure seas, and clear blue skies. It is noon, with the sun high in the sky, casting bright and warm rays upon everything, illuminating this beautiful land.
The protagonist stands tall, wielding their weapon, exuding confidence and determination in the wake of victory. They wear a smile, their eyes gleaming with joy and contentment.
Ed stands beside the protagonist, likewise displaying a joyful expression of triumph. The two stand shoulder to shoulder, radiating trust and friendship.
In this victorious land, the protagonist declares, "We did it! The forces of darkness have finally been defeated!" Ed responds, "Yes, we have triumphed over evil! This land is once again filled with peace and hope!"
The music is grand and solemn, embodying an atmosphere of victory and freedom. The sound effects are mighty, with instruments and voices gradually rising, symbolizing the immense power of justice. Natural sounds also intermingle, as bird songs and the sound of the waves intertwine, adding vibrancy to this moment of triumph.

\begin{figure}[h]
  \centering
  \includegraphics[width=1.0\textwidth]{figures/SPP扩写.png}
  \tiny
  \caption{'Trivia Creative Writing task example'}
  \label{fig:trivia creative writing}
\end{figure}
